# Supplementary material for: SpatialTracker: Tracking Any 2D Pixels in 3D Space
Source: arXiv:2404.04319 source file (2024-04-05)
Supplement: Supplementary file 1 [file 7.appendix.tex]

\appendix

\setcounter{equation}{0}
\setcounter{table}{0}
\setcounter{figure}{0}

\section*{Appendix}
